# Supplementary material for: DiffuSIA: A Spiral Interaction Architecture for Encoder-Decoder Text Diffusion
Source: arXiv:2305.11517 source file (2023-05-19)
Supplement: Supplementary file 1 [file appendix.tex]

\section{Experimental Settings}

  \subsection{Datasets} \label{sec-datasets}

    \begin{table}[!hbt]
      \small
      \centering
      \setlength{\tabcolsep}{2.4pt}
      \begin{tabular}{c|c|c|c|c}
      \toprule
        \multicolumn{2}{c|}{Datasets}                                  &   Train   &   Valid   &  Test    \\
      \hline
        \multicolumn{2}{c|}{\citet{DBLP:conf/ijcai/HuCL0MY19}}         &  311,725  &  5,000    &  5,000  \\
      \hline
        \multirow{3}{*}{\citet{DBLP:conf/emnlp/OuchiT16}}   &  Len-5   &  461,120  &  28,570   &  32,668  \\
                                                            &  Len-10  &  495,226  &  30,974   &  35,638  \\
                                                            &  Len-15  &  489,812  &  30,815   &  35,385  \\
      \bottomrule
      \end{tabular}
      \caption{Statistics of the two benchmarks evaluated in this paper.}
      \label{tab-data}
    \end{table}

    % We evaluated our proposed methods on two Ubuntu IRC benchmarks.
    % One was released by \citet{DBLP:conf/ijcai/HuCL0MY19}, in which both speaker and addressee labels was provided for each utterance.
    % % The corpus consists of a huge amount of records including response utterances, interlocutor IDs and their posting time.
    % The other benchmark was released by \citet{DBLP:conf/emnlp/OuchiT16}.
    % Here, we adopted the version shared in \citet{DBLP:conf/emnlp/LeHSYBZY19} for fair comparison. %in which sessions without a single addressee ground truth and sessions with one or more blank utterance were filtered out.
    % The conversation sessions were separated into three categories according to the session length (Len-5, Len-10 and Len-15) following the splitting strategy of previous studies \cite{DBLP:conf/emnlp/OuchiT16,DBLP:conf/aaai/ZhangLPR18,DBLP:conf/emnlp/LeHSYBZY19}.
    Table~\ref{tab-data} presents the statistics of the two benchmarks evaluated in our experiments.

  \subsection{Baseline Models} \label{sec-baselines}    
    We compared our proposed model with as many MPC generative models as possible.
    Considering that there are only a few research papers in this field, several recent advanced models were also adapted to provide sufficient comparisons following \citet{DBLP:conf/acl/GuTTLHGJ22}.
    Finally, we compared with (1) non-graph-based models including RNN-based Seq2Seq~\cite{DBLP:conf/nips/SutskeverVL14}, Transformer~\cite{DBLP:conf/nips/VaswaniSPUJGKP17}, GPT-2~\cite{radford2019language} and BART~\cite{DBLP:conf/acl/LewisLGGMLSZ20},
    as well as (2) graph-based models including GSN~\cite{DBLP:conf/ijcai/HuCL0MY19} and HeterMPC~\cite{DBLP:conf/acl/GuTTLHGJ22} as follows. %BERT~\cite{DBLP:conf/naacl/DevlinCLT19}
    
    \textbf{(1) RNN-based Seq2Seq} \cite{DBLP:conf/nips/SutskeverVL14} took all utterances except the target utterance to generate as input, which were sorted according to their posting time and concatenated. Thus, structured conversations were converted into sequential ones. Seq2Seq modeling with attention was performed as that in \citet{DBLP:conf/nips/SutskeverVL14,DBLP:journals/corr/BahdanauCB14} on the concatenated utterances.
    \textbf{(2) Transformer} \cite{DBLP:conf/nips/VaswaniSPUJGKP17} took the same input utterances as those used for the Seq2Seq model.
    \textbf{(3) GPT-2} \cite{radford2019language} was a uni-directional pre-trained language model. Following its original concatenation operation, all context utterances and the response were concatenated with a special \texttt{[SEP]} token as input for encoding. 
    % \textbf{(4) BERT} \cite{DBLP:conf/naacl/DevlinCLT19} concatenated all context utterances and the response similarly as those for GPT-2. To adapt BERT for response generation, a special masking mechanism was designed to avoid response information leakage during encoding. Concretely, each token in the context utterances attended to all tokens in the context utterances, while each token in the response cannot attend to future tokens in the utterance. 
    \textbf{(4) BART} \cite{DBLP:conf/acl/LewisLGGMLSZ20} was a denoising autoencoder using a standard Tranformer-based architecture, trained by corrupting text with an arbitrary noising function and learning to reconstruct the original text. In our experiments, a concatenated context started with <s> and separated with </s> were fed into the encoder, and a response were fed into the decoder.
    \textbf{(5) GSN} \cite{DBLP:conf/ijcai/HuCL0MY19} made the first attempt to model an MPC with a homogeneous graph. The core of GSN was an utterance-level graph-structured encoder.
    \textbf{(6) HeterMPC} \cite{DBLP:conf/acl/GuTTLHGJ22} achieved the state-of-the-art performance on MPCs. It proposed to model the complicated interactions between utterances and interlocutors in MPCs with a heterogeneous graph, where two types of graph nodes and six types of edges are designed to model heterogeneity. Two versions of HeterMPC were provided that were initialized with BERT and BART respectively. The latter was adopted in this paper which showed better performance.

  \subsection{Implementation Details} \label{sec-details}
    Model parameters were initialized with pre-trained weights of \emph{bert-base-uncased} released by \citet{DBLP:conf/emnlp/WolfDSCDMCRLFDS20}. 
    % The word embedding table was shared between the encoder and decoder.
    The AdamW method~\cite{DBLP:conf/iclr/LoshchilovH19} was employed for optimization. 
    The learning rate was initialized as $6.25e\text{-}5$ and was decayed linearly down to $0$. 
    The max gradient norm was clipped down to $1.0$.
    The batch size was set to $16$ with $8$ gradient accumulation steps.
    The maximum utterance length was set to $50$. 
    The number of layers for initializing utterance representations $L_1$ was set to 9, and the number of layers for heterogeneous graph iteration $L_2$ was set to 3. 
    $L_1$ and $L_2$ were validated on the validation set.
    The number of decoder layers $L_3$ was set to 6, achieving the best performance out of \{2, 4, 6, 8\} on the validation set.
    The strategy of greedy search was performed for decoding. 
    The maximum length of responses for generation was also set to $50$. 
    All experiments were run on a single GeForce RTX 2080 Ti GPU. 
    The maximum number of epochs was set to 15, taking about 40 hours. 
    The validation set was used to select the best model for testing. 
    All code was implemented in the PyTorch framework\footnote{https://pytorch.org/} and will be published to help replicate our results. %are published to help replicate our results.~\footnote{https://github.com/lxchtan/HeterMPC}
